# Supplementary material for: Semantic Preserving Generative Adversarial Models
Source: arXiv:1910.02804 source file (2019-10-07)
Supplement: Supplementary file 1 [file aaaiSuppelmentary.tex]

\begin{figure*}[h]
    \includegraphics[width=0.4\textwidth,height=0.25\textwidth]{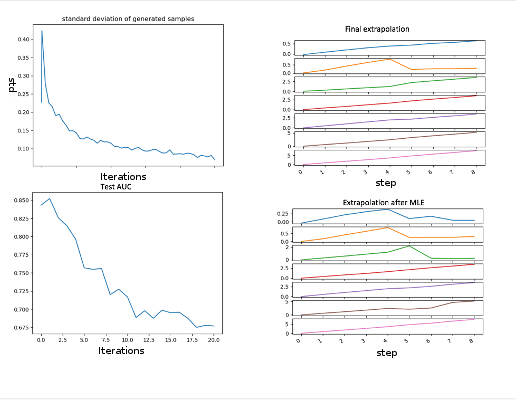}
  \caption{Generation and extrapolation using only 16 training points}
  \label{fig:lines}
\end{figure*}
